# Supplementary material for: Calculating modules in contextual logic program refinement
Source: arXiv:cs/0608110 source file (2006-08-29)
Supplement: Supplementary file 1 [file appendix.tex]

\appendix
\section{Refinement Laws}
\label{ax}

%This appendix includes refinement laws used throughout the paper.

Note that disjunction and parallel conjunction are commutative
(sequential conjunction is not), and all three are associative and
idempotent, \ie, 
\[
	S \lor S \refeq S \land S \refeq S,S \refeq S
\]

\COMMENT{
\subsection{Lifting}
\label{lifting}

{\ReftLaw Lift conjunction \thlabel{lift:conj}}
\[
     \Spec{P \land Q} \refeq \Spec{P} \land \Spec{Q}
\]

{\ReftLaw Lift disjunction \thlabel{lift:disj}}
\[
     \Spec{P \lor Q} \refeq \Spec{P} \lor \Spec{Q}
\]
}

%{\ReftLaw Lift existential \thlabel{lift:exists}}
%\[
     %\Spec{(\exists X @ P)} \refeq (\exists X @ \Spec{P})
%\]

\COMMENT{
{\ReftLaw Lift universal \thlabel{lift:all}}
\[
     \Spec{(\all X @ P)} \refeq (\all X @ \Spec{P})
\]

{\ReftLaw Distribute parallel through disjunction \thlabel{dist:para:disj}}
\[
     S \land (T \lor U) \refeq (S \land T) \lor (S \land U)
\]
}

\COMMENT{
\subsection{Distribution}
\label{dist:assoc}

{\ReftLaw Distribute disjunction through parallel \thlabel{dist:disj:para}}
\[
     S \lor (T \land U) \refeq (S \lor T) \land (S \lor U)
\]

{\ReftLaw Distribute sequential through disjunction  \thlabel{dist:seq:disj}}
\[
     S , (T \lor U) \refeq (S , T) \lor (S , U)
\]

{\ReftLaw Parallel conjunction associativity \thlabel{assoc:conj}}
\[
     S \land (T \land U) \refeq (S \land T) \land U
\]
}

\COMMENT{
{\ReftLaw Parallel into sequential \thlabel{pand:into:seq}}
\[
    S \land (T,U) \refsto T,(S \land U)
\] 
\Proof
\begin{derivation}
	\step{S \land (T,U) \refsto T,(S \land U)}
	\trans{\iff}{\refdefn{pred:refsto}}
	\step{ok.S \land ok.T \land (ef.T \imp ok.U) \entails}
		\step{\t1 ok.T \land (ef.T \imp ok.S \land ok.U) \land}
		\step{\t1 ef.S \land ef.T \land ef.U \iff ef.T \land ef.S \land ef.U}
	\trans{\iff}{simplify}
	\step{ok.S \land ok.T \land (ef.T \imp ok.U) \entails}
		\step{\t1 ef.T \imp ok.U \rcpqed}
\end{derivation}
}

%\subsection{Extend scope}

\COMMENT{
{\ReftLaw Extend scope of existential over parallel conjunction 
	\thlabel{exists:extend:scope:para}}
\[
	(\exists X @ S) \land T \refeq (\exists X @ S \land T) \\
    \Proviso{$X \nfi T$}
\]   
\Proof
Since $X \nfi T$, we deduce that $X \nfi ok.T$ and $X \nfi ef.T$.
\begin{derivation}
	\step{(\exists X @ S) \land T \refeq (\exists X @ S \land T)}
	\trans{\iff}{\refdefn{pred:refsto}}
	\step{(\all X @ ok.S) \land ok.T \entails}
		\step{\t1 (\all X @ ok.S \land ok.T) \land}
		\step{\t1 (\exists X @ ef.S) \land ef.T 
				  \iff (\exists X @ ef.S \land ef.T)}
	\trans{\iff}{extend scope of (predicate) quantification, from proviso} 
	\step{(\all X @ ok.S \land ok.T) \entails}
		\step{\t1 (\all X @ ok.S \land ok.T) \land}
		\step{\t1 (\exists X @ ef.S \land ef.T) 
				  \iff (\exists X @ ef.S \land ef.T) \rcpqed}
\end{derivation}
}

\COMMENT{
{\ReftLaw Extend scope of existential over disjunction
	\thlabel{exists:extend:scope:disj}}
\[
	(\exists X @ S) \lor T \refeq (\exists X @ S \lor T) \\
    \Proviso{$X \nfi T$}
\]
}

%{\ReftLaw Extend scope of existential over sequential conjunction (left)
	%\thlabel{exists:extend:scope:seqL}}
%\[
	%(\exists X @ S), T \refeq (\exists X @ S,T) \\
    %\Proviso{$X \nfi T$}
%\]     

\COMMENT{
\Proof
Similar to the proof of \ref{exists:extend:scope:para} \tqed.
}
\COMMENT{
{\ReftLaw Extend scope of existential over sequential conjunction (right)
	\thlabel{exists:extend:scope:seqR}}
\[
    T, (\exists X @ S) \refeq (\exists X @ T,S) \\
    \Proviso{$X \nfi T$}
\]
}

%\subsection{Specifications}

\COMMENT{
{\ReftLaw Equivalent specifications \thlabel{equiv:specs}}
\[
    \Rule{\G \entails P \iff Q}
        {\G \inctx \Spec{P} \refeq \Spec{Q}}
\]
}

\COMMENT{
{\ReftLaw Eliminate/introduce specification 
\thlabel{intro:spec} \thlabel{elim:redund:spec}}
\[
    \Rule{\G \entails A}
        {\G \inctx \Spec{A} \land S \refeq S}
\]
}

%{\ReftLaw Eliminate/introduce specification 2 
%\thlabel{intro:spec2} \thlabel{elim:redund:spec2}}
% cf. create inv.
%\[
    %A \inctx {\Spec{A} , S \refeq S}
    %\Rule{\G \entails A}
        %{\G \inctx \Spec{A} , S \refeq S}
%\]

\COMMENT{
{\ReftLaw Implied specification \thlabel{implied:spec}}
\[
    \Rule{\G \entails P \imp Q}
        {\G \inctx \Spec{P} \refeq \Spec{P \land Q}}
\]
}

\COMMENT{
{\ReftLaw Assumption in context \thlabel{ass:spec:refsto}}
\[  
    \Rule{\G \entails (P \iff Q)}
		{\G \inctx \Spec{P} \refsto \Spec{Q}}
\]

{\ReftLaw Assumption in context \thlabel{ass:spec:refsto:old}}
\[  
    \Rule{A \entails (P \iff Q)}
		{\Ass{A}, \Spec{P} \refsto \Ass{A}, \Spec{Q}}
\]
}

%\subsection{Assumptions}

\COMMENT{
{\ReftLaw Introduce assumption from context \thlabel{intro:ass:old}}
\[
    \Rule{A}
        {S \refeq \Ass{A},S}
\]
}

%{\ReftLaw Introduce assumption from context \thlabel{intro:ass}}
%\[
    %\Rule{\G \entails A}
        %{\G \inctx S \refeq \Ass{A},S}
%\]

\COMMENT{
{\ReftLaw Remove assumption \thlabel{remove:ass}}
\[
	\Ass{A},S \refsto S
\]
}

\COMMENT{
{\ReftLaw Weaken assumption \thlabel{weaken:ass}}
\[
	\Rule{\G \entails A \imp B}
	{\G \inctx \Ass{A} \refsto \Ass{B}}
\]
}

%\subsection{Parallel specifications}

\COMMENT{
{\ReftLaw Parallel specification in context \thlabel{para:incontext}}
\[
    \Rule{I \imp (B \refsto B'); ok.B \imp ok.B'}
        {\Spec{I} \land B \refsto \Spec{I} \land B'}
\]

{\ReftLaw Discharge parallel specification \thlabel{discharge:para}}
\[
	\Rule{\G \entails (ok.S \land ef.S) \imp P } 
		{\G \inctx S \land \Spec{P} \refeq S }
\]
}

\COMMENT{
{\ReftLaw Parallel specifications \thlabel{para:ctx:para}}
\[
    \Rule{\G \entails P \imp (Q \iff Q')}
		{\G \inctx \Spec{P} \land \Spec{Q} \refsto \Spec{P} \land \Spec{Q'}}
\]
}
\COMMENT{
\Proof 
\begin{derivation}
	\step{\Spec{P} \land \Spec{Q}}
	\trans{\refeq}{\reflaw{lift:conj}}
	\step{\Spec{P\land Q}}
	\trans{\refeq}{\reflaw{equiv:specs} from hypothesis}
	\step{\Spec{P\land Q'}}
	\trans{\refeq}{\reflaw{lift:conj}}
	\step{\Spec{P} \land \Spec{Q'}}
\end{derivation}

}

%\subsection{Parameterised commands}
%\label{ax:pcmd}

\COMMENT{
{\ReftLaw Parameterise \thlabel{parameterise}}
\[
    \replace{S}{V}{T} \refeq (V \prm S)(T)
\]

{\ReftLaw Unfold recursion \thlabel{rec:unfold}}
\[
    (\re p @ V \prm \C(V, p) \er)(X) \refeq 
	\C(X, (\re p @ V \prm \C(V, p) \er))
\]
}

%{\ReftLaw Recursion introduction \label{general:rec:intro:rc} \\
%Suppose $pc:PCmd$ is a parameterised command; $(\_ \prec \_): Term \rel
%Term$ is a well-founded relation; and
%$id$ is a fresh name;
%and environment $\rho' =
%\rho \union \{id \mapsto (\re id @ V \prm C(id) \er)\}$.}
\COMMENT{
\[
    \Rule{(\all Y:Term @ \Ass{Y \wflt X}, pc(Y) \refsto id(Y)) \imp
        pc(X) \refsto \C(id)}
    {pc \refstorho (\re id @ X \prm \C(id) \er)}
\]
}

\COMMENT{
\subsection{Skip and failure Laws}

We have
\[
	\Skip == \Spec{true} == \Ass{true} \\
	\fail == \Spec{false} \\
	\abort == \Ass{false}
\]

{\ReftLaw Eliminate skip sequential \thlabel{elim:skip}}
\[
    \Skip, S \refeq S
\]

{\ReftLaw Eliminate skip parallel \thlabel{elim:skip:para}}
\[
    \Skip \land S \refeq S
\]

{\ReftLaw Eliminate failure \thlabel{elim:fail}}
\[
    S \lor \fail \refeq S
\]

{\ReftLaw Abort inclusion \thlabel{ass:abort}}
\[
    \Ass{A}, \abort \refeq \abort
\]
}
\COMMENT{
\Proof
\begin{derivation}
	\step{\Ass{A}, \abort \refeq \abort}
	\trans{\iff}{\refdefn{pred:refeq}}
	\step{(ok.A \land false) \iff false \rcpqed}
\end{derivation}

}
%\subsection{Case analysis}

\COMMENT{
{\ReftLaw Case analysis from assumption \thlabel{case:analysis:ass}}
\[
	\Rule{A \imp (P \lor Q)}
	{\Ass{A}, S \refsto \Ass{A}, (\Spec{P},S \lor \Spec{Q},S)}
\]
}

\COMMENT{
{\ReftLaw Case analysis to parallel \thlabel{case:anal}}
\[
    \Rule{\G \entails A \lor B}
        {\G \inctx S \refeq (\Spec{A} \land S) \lor (\Spec{B} \land S)}
\]
\Proof
\begin{derivation}
	\step{S}
	\trans{\refeq}{\reflaw{intro:spec} from hypothesis}
	\step{\Spec{A \lor B} \land S}
	\trans{\refeq}{\reflaw{lift:disj}}
	\step{(\Spec{A} \lor \Spec{B}) \land S}
	\trans{\refeq}{\reflaw{dist:para:disj}}
	\step{(\Spec{A} \land S) \lor (\Spec{B} \land S)}
\end{derivation}
}

%{\ReftLaw Case analysis to sequential \thlabel{case:anal:seq}}
%\[
    %\Rule{\G \entails A \lor B}
        %{\G \inctx S \refsto (\Spec{A} , S) \lor (\Spec{B} , S)}
%\]
\COMMENT{
\Proof
From \reflaw{case:anal} and \reflaw{para:to:seq}. \tqed
}

\COMMENT{
\subsection{Context}

{\ReftLaw Specification in context \thlabel{ctx:seq:spec}}
\[
    \Rule{\G \land P \inctx (T \refsto T')}
        {\G \inctx \Spec{P},T \refsto \Spec{P},T'}
\]

{\ReftLaw Context for parallel specification \thlabel{weaken:para:ax}}
\[
    \Rule{\G \entails (ok.S \land ef.S) \imp (P \iff P')} 
        {\G \inctx S \land \Spec{P} \refsto S \land \Spec{P'} }
\]
}

%\subsection{Other laws}

\COMMENT{
{\ReftLaw Parallel to sequential \thlabel{para:to:seq}}
\[
	S \land T \refsto S,T
\]
}

\COMMENT{
{\ReftLaw Sequential to parallel \thlabel{exists:seq:para}}
\[
	\Rule{(\exists X @ P)}
		{(\exists X @ \Spec{P}, S) \refeq (\exists X @ \Spec{P} \land S)}
	\Proviso{$X$ does not occur free in $ok.S$}
\]
}

\COMMENT{
\Proof
\begin{derivation}
	\step{(\exists X @ \Spec{P}, S) \refeq (\exists X @ \Spec{P} \land S)}
	\trans{\equiv}{\refdefn{pred:refeq}}
	\step{(\all X @ P \imp ok.S) \equiv (\all X @ ok.S) \land}
	\step{(\all X @ P \imp ok.S) \entails}
		\step{\t1 (\exists X @ P \land ef.S) \iff (\exists X @ P \land ef.S)}
	\trans{\equiv}{simplification}
	\step{(\all X @ P \imp ok.S) \equiv (\all X @ ok.S)}
	\trans{\equiv}{proviso $X \nfi ok.S$}
	\step{((\exists X @ P) \imp ok.S) \equiv ok.S}
	\trans{\equiv}{hypothesis}
	\step{ok.S \equiv ok.S \rcpqed}
\end{derivation}
}

\COMMENT{
{\ReftLaw One-point law (existential) \thlabel{one:pt:exists}\\
Provided $X \nfi E$,}
\[
	(\exists X @ \Spec{X = E}, S) \refeq \replace{S}{X}{E}
\]

\Proof
\begin{derivation}
	\step{\textstyle (\exists X @ \Spec{X = E}, S) \refeq \replace{S}{X}{E}}
	\trans{\equiv}{\refdefn{pred:refeq}}
	\step{\textstyle (\all X @ X = E \imp ok.S) \equiv ok.\replace{S}{X}{E} \land}
	\step{(\all X @ X = E \imp ok.S) \entails }
		\step{\textstyle 
			\t1 (\exists X @ X = E \land ef.S) \iff ef.\replace{S}{X}{E}}
	\trans{\equiv}{One-point law existential, one-point law universal
	from $X \nfi E$}
	\step{\textstyle \replace{ok.S}{X}{E} \equiv ok.\replace{S}{X}{E} \land}
	\step{\textstyle\replace{ok.S}{X}{E} \entails}
		\step{\textstyle \t1 \replace{ef.S}{X}{E} \iff ef.\replace{S}{X}{E}
			\rcpqed}
\end{derivation}
}

\COMMENT{
{\ReftLaw One-point law (existential) over parallel 
\thlabel{one:pt:exists:para}\\
Provided $X \nfi E$,}
\[
	(\exists X @ \Spec{X = E} \land S) \refsto \replace{S}{X}{E}
\]
\Proof From \reflawN{para:to:seq} and \reflawN{one:pt:exists}. \tqed
}

\COMMENT{
{\ReftLaw Remove unneeded variable \thlabel{unneeded:var}}
\[
    \Rule{\exists X @ P}
         {(\exists X @ \Spec{P} \land S) \refeq S} \\
    \mbox{\hskip 5mm \it Provided $X$ does not occur free in $S$}
\]

{\ReftLaw Join assumptions over parallel \thlabel{join:ass:over:parallel}}
\[
    \Ass{A}, (S \land (\Ass{B}, T)) \refeq 
    \Ass{A \land B}, (S \land T)
\]
}

\COMMENT{
\subsection{Dubious laws}

{\ReftLaw Uninstantiated abortion \thlabel{exists:abort}}
\[
    \Rule{\lnot(\all X @ A)}
    {(\exists X @ \Ass{A}, S) \refeq \abort}
\]

Proof: DO ME
}

\COMMENT{
\subsection{Monotonicity}

{\ReftLaw Monotonicity of parallel \thlabel{mono:parallel}}
\[
    \Rule{ S \refsto S';\ T \refsto T'}
         { S \land T \refsto S' \land T' }
\]

{\ReftLaw Monotonicity of sequential \thlabel{mono:seq}}
\[
    \Rule{ S \refsto S';\ T \refsto T'}
         { S , T \refsto S' , T' }
\]

{\ReftLaw Monotonicity of disjunction \thlabel{mono:disj}}
\[
    \Rule{ S \refsto S';\ T \refsto T'}
         { S \lor T \refsto S' \lor T' }
\]

{\ReftLaw Monotonicity of existential \thlabel{mono:exists}}
\[
    \Rule{ S \refsto S'}
         { (\exists X @ S) \refsto (\exists X @ S')}
\]

{\ReftLaw Monotonicity of universal \thlabel{mono:all}}
\[
    \Rule{ S \refsto S'}
         { (\all X @ S) \refsto (\all X @ S')}
\]
}

\COMMENT{
\section{Predicate Laws}
\label{pred:laws}

This appendix lists some of the propositional and predicate laws used in the
thesis.
We include a proof for
\reflawN{imp:all:imp}
since it is not listed in \cite{Gries:94}.
%and \reflawN{imp:exists:iff}.
}

\COMMENT{
{\ReftLaw ~ \thlabel{imp:iff}}
\[
	(A \land B \equiv A \land C) \equiv (A \entails (B \iff C))
\]
}

\COMMENT{
{\ReftLaw Split universal quantification \thlabel{split:forall} \\
Provided $N > 0$,}
\[
    (\all i:1..N @ \P(i)) \iff (\P(1) \land (\all i: 2..N @ \P(i))
\]

{\ReftLaw Shift range \thlabel{shorten:range:ax}}
\[
    (\all i :2..N @ \P(V,L,i)) \iff (\all i :1..N-1 @ \P(V,L,i+1)) \\
\]
This is an instance of the more general property
\[
	(\all i:S @ \P) \iff (\all j: T @ \P[f(j)/i])
	\Proviso{$S = f\limg T \rimg$}
\]
where $S = 2..N$ and $f = (\lambda x @ x +1)$.
}

\COMMENT{
{\ReftLaw ~ \thlabel{plus1:tail:ax}} 
\[
    list(L) \land L = \HT \land i \in 1.. \#T \imp \\
        \t1 L(i+1) = T(i) \land L(1) = H
\]
\Proof

{\ReftLaw ~ \thlabel{reduce:scope:univ:imp}}
\[
    (\all X @ P \imp Q) \equiv (\exists X @ P) \imp Q \\
	\Proviso{X \nfi Q}
\]

{\ReftLaw ~ \thlabel{imp:exists}}
\[
    %\Rule{\replace{E}{X}{T}}{(\exists X @ E)}
    \replace{E}{X}{T} \entails (\exists X @ E)
\]
}

\COMMENT{
{\ReftLaw ~ \thlabel{imp:all}}
\[
    (\all X @ E) \entails \replace{E}{X}{T}
\]

{\ReftLaw ~ \thlabel{imp:all:imp}}
\[
    \Rule{A \imp B}
		{(\all X @ A) \imp (\all X @ B)}
\]
}

\COMMENT{
\Proof 
\begin{derivation}
	\step{(\all X @ A) \imp (\all X @ B)}
	\trans{\iff}{from hypothesis}
	\step{(\all X @ A \land B) \imp (\all X @ B)}
	\trans{\iff}{distribute quantification}
	\step{(\all X @ A) \land (\all X @ B) \imp (\all X @ B) \rcpqed}
\end{derivation}
}

\COMMENT{
{\ReftLaw ~ \thlabel{imp:exists:iff}}
\[
    \Rule{A \iff B}
		{(\exists X @ A) \iff (\exists X @ B)}
\]
\Proof 
\begin{derivation}
	\step{(\exists X @ A) \iff (\exists X @ B)}
	\trans{\iff}{from hypothesis}
	\step{(\exists X @ A) \iff (\exists X @ A) \rcpqed}
\end{derivation}
}
